# Supplementary material for: Phonon dispersion of MoS$_2$
Source: arXiv:1809.03381 ancillary file (2018-09-10)
Supplement: Supplementary file 1 [file SupplementalMaterial_PhononDispersionOfMoS2.pdf]

# Supplemental material for
# Phonon dispersion of $MoS_2$

Hans Tornatzky,[1,*] Roland Gillen,[2] Hiroshi Uchiyama,[3] and Janina Maultzsch[2]

[1] *Institut für Festkörperphysik, Technische Universität Berlin Hardenbergstr. 36, 10623 Berlin, Germany*
[2] *Department Physik, Friedrich-Alexander-Universität Erlangen-Nürnberg, Staudtstr. 7, 91058 Erlangen, Germany*
[3] *Japan Synchrotron Radiation Research Institute (JASRI/SPring-8), 1-1-1 Kouto, Sayo, Hyogo 679-5198 Japan*
(Dated: September 10, 2018)

## METHODS

### Experimental setup

Our inelastic X-ray spectra were recorded at beamline 35XU at the SPring-8 (Japan). A beam with a photon energy of 17.7935 keV with a spectral width of $\lesssim 3$ meV (full width of half maximum, FWHM) was obtained by using a liquid-nitrogen cooled Si (111) high heat load pre-monochromator, reducing the FWHM to $\approx 1$ eV. The final width was created with a near-backscattering main monochromator of which the Si (999) reflex was used. The beam was then focused onto the sample with a spot size of $75 \times 63\,\mu\text{m}^2$, enabling us to select a single crystalline domain of the bulk $MoS_2$ crystal. The scattered photons were analyzed by an array of 3x4 bent Si (111) analyzers, attached to the 10 m monochromator arm. A detailed description of the beamline can be found in Ref. [1].

The measurements were performed by keeping the scattering wave vector $Q$ (and thereby the phonon wave vector $q$) constant and scan the energy by varying the temperature of the backscattering main monochromator. The twelve analyzers were kept at a fixed energy (i.e. temperature). To verify that no significant energy shifts of analyzers and main monochromator have occurred, Stokes-anti-Stokes pairs of inelastically scattered photons were measured between most of the energy scans. The measurements were performed in reflection geometry for $\Gamma A$ longitudinal and all out-of-plane transverse modes and in transmission for $\Gamma M$, $\Gamma K$ and $KM$ longitudinal and in-plane transverse modes. To record signal from low-intensity modes, momentum resolution was set to $0.75\,\text{nm}^{-1}$.

The sample is a synthesized crystal (HQ graphene, Netherlands) with a thickness of about $150\,\mu$m to match the attenuation length of the used X-rays in $MoS_2$, yielding the best trade-off between high absorption and low scattering in a transmission setup.

Raman measurements were performed on a Horiba LabRAM HR with excitation wavelengths of 633 nm and 457 nm. An ultra-low frequency notch filter was used with the 633 nm laser to observe the shear mode ($E_{2g}$).

All measurements were taken in ambient conditions.

### Computational approach

We calculated the theoretical phonon band structure within the frame of density functional perturbation theory (DFPT) on the level of the generalized gradient approximation in the Perdew-Burke-Ernzerhof flavor (GGA-PBE) as implemented into the Quantum Espresso suite [2]. Long-range non-covalent interactions were included through the semi-empirical DFT-D3 correction with Becke-Johnson damping [3],

$$E^{D3} = \frac{1}{2}\sum_A \sum_B \left( C_6^{AB} \frac{s_6}{R_{AB}^6 + f^6} + C_8^{AB} \frac{s_8}{R_{AB}^8 + f^8} \right),$$

where $R_{AB}$ is the distance between atom $A$ in a central unit cell and an atom $B$ in the crystal. We included all atoms within a cutoff distance of 100 Å from the center of the central unit cell in the sum over $B$. $C_n^{AB}$ is the $n$-th order dispersion coefficient for the pair of atoms $A$ and $B$. $f = a_1 R_{AB}^0 + a_2$ is a damping constant, with a 'covalent distance' $R_{AB}^0 = \sqrt{C_8^{AB}/C_6^{AB}}$ [3]. Here, we used our own set of parameters ($s_6$=1.0, $s_8$=0.9184, $a_1$=0.5484, $a_2$=2.156 Å), which was fitted to reproduce the experimental lattice constants of a wide variety of layered and bulk materials and had been used previously [4–6] with great success. The Mo($3s$,$3p$,$3d$,$4s$) and the S($3s$,$3p$) states were treated as valence electrons using multi-projector optimized normconserving Vanderbildt (ONCV) pseudopotentials [7, 8] with a cutoff of 120 Ry. All reciprocal space integrations were performed by a discrete $q$ point sampling of 12x12x4 $q$ points in the Brillouin zone. We fully optimized the atomic positions and cell parameters until the residual forces between atoms and the cell stress were smaller than 0.001 eV/Å and 0.01 GPa, respectively. The threshold for the total energy was set to $10^{-14}$ Ry, which ensured tightly converged interatomic forces for the geometry optimization and of the ground state density and wavefunctions for the DFPT calculations. The phonon band structure was obtained through Fourier interpolation using the explicitly calculated phonon frequencies on a regular grid of 12x12x4 $q$ points. The contributions to the dynamical matrix from the D3 corrections were fully included in the phonon calculations.

We find a small overestimation of our predicted frequencies of the out-of-plane acoustic (ZA) mode com-

pared to the IXS measurements. While the deviation is within the margin of error in our measurements, we note that this mode is particularly difficult to converge with the cutoff energy of the plane-wave expansion that we use in our calculations, due to the weak forces between the rigidly oscillating layers. This situation is similar to the ZA modes in graphite and layered boron nitride. A D3 correction to an exchange-correlation approximation with a higher quality intrinsic prediction of structural and vibrational properties might lead to a further improvement but requires a suitable set of 'fitting' parameters to seamlessly connect the long-range non-covalent interactions from the correction with the already existing short-range interactions from the underlying exchange-correlation functional.

## Raman spectroscopy

Raman spectra of the same sample as used in the IXS measurements were acquired to complement the measured IXS spectra (see Fig. S 1). The spectrum at low wavenumbers was acquired using an ultra low frequency filter with 633 nm excitation wavelength. Since the higher-frequency first-order modes are not easily deconvoluted from the resonance-induced strong higher-order background, an excitation of 457 nm was chosen for the determination of the high-energy optical Raman modes ($E_{2g}$ and $A_{1g}$). We assign non-labeled peaks in Fig. S 1 to higher-order Raman scattering processes. We did not observe the defect-enabled (first order) "LA" peak ($A_1'$ or $A_2'$ at K and $B_{3u}/A_g$ at M) at $\approx 230\,\mathrm{cm}^{-1}$, see inset to Fig. S 1, which confirms a good crystal quality [9, 10].

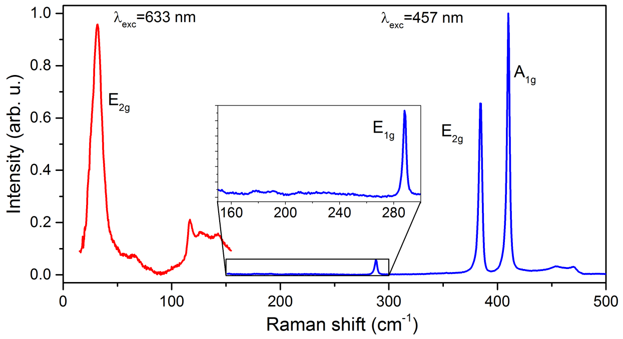


FIG. S 1: Raman spectra of the $MoS_2$ crystal used for the IXS measurements. The red (blue) spectrum is acquired with 633 nm (457 nm) excitation wavelength.

## Simulation of IXS intensities

To supplement our experimental data and obtain more insight into the observed relative scattering intensities, we simulated the dynamical structure factor of $MoS_2$ for inelastic X-ray (and neutron) scattering. Following Ref. [11], we compute the one-phonon contribution to the dynamical structure factor for a reduced phonon wavevector $\mathbf{q}$ through

$$S(\mathbf{q},\omega)_{hkl} \propto \sum_{j}^{3N_{at}} \left| \sum_{d} \frac{f_d\left(\mathbf{G}_{hkl}+\mathbf{q}\right)}{\sqrt{2M_d}} e^{-W_d(\mathbf{G}_{hkl}+\mathbf{q})} \left(\mathbf{G}_{hkl}+\mathbf{q}\right)\cdot \mathbf{e}_{\mathbf{q}jd}\, e^{i(\mathbf{G}_{hkl}+\mathbf{q})\cdot \mathbf{x}_d} \right|^2 F^{\mathrm{DHO}}_{\mathbf{q}j}(\omega) \tag{1}$$

where $\mathbf{x}_d$ and $M_d$ are the position and mass of atom $d$ in the unit cell, respectively, $\mathbf{e}_{\mathbf{q}jd}$ is the displacement of atom $d$ due to phonon mode $j$, and $\mathbf{G}_{hkl}$ is the reciprocal lattice vector corresponding to the Bragg peak ($h$ $k$ $l$). $N_{at}$ is the number of atoms in the unit cell, $e^{2W_d}$ is the Debye-Waller factor of atom $d$, while $f_d$ is the wavevector-dependent form factor and readily available in tabulated form.

We approximate the spectral shape and temperature dependence of the structure factor due to electron-phonon and phonon-phonon scattering by a damped harmonic oscillator (DHO) model [12]

$$F^{\mathrm{DHO}}_{\mathbf{q}j}(\omega) = \frac{4\omega}{\pi\left(1-e^{\hbar\omega/k_BT}\right)} \frac{\gamma_{\mathbf{q}j}}{\left(\omega^2-\Omega^2_{\mathbf{q}j}\right)^2+4\omega^2\gamma^2_{\mathbf{q}j}},$$

where $\omega_{\mathbf{q}j}$ and $\gamma_{\mathbf{q}j}$ are the angular frequency and linewidth of phonon mode $j$ at wavevector $\mathbf{q}$, respectively. $\Omega^2_{\mathbf{q}j} = \omega^2_{\mathbf{q}} + \gamma^2_{\mathbf{q}j}$ is the effective frequency of the phonon mode. The Debye-Waller Factor $e^{2W_d}$ is potentially important in our case as it might be different for different atoms/species and cause further qualitative differences of the phonon modes, *e.g.*, modes with smaller or larger oscillations of the molybdenum atoms, in terms of inelastic scattering of X-rays. We thus explicitly included the Debye-Waller factor, with [11]

$$W_d\left(\mathbf{G}_{hkl}+\mathbf{q}\right)=\frac{\hbar}{4M_dN_q}\sum_{\mathbf{q}}\sum_{j}^{3N_{at}}\frac{1}{\omega_{\mathbf{q}j}}\left|\left(\mathbf{G}_{hkl}+\mathbf{q}\right)\cdot\mathbf{e}_{\mathbf{q}jd}\right|^2\coth\left(\frac{\hbar\omega_{\mathbf{q}j}}{2k_BT}\hbar\right),, \quad (2)$$

which requires a sum over $N_q$ vectors in the first Brillouin zone of the crystal. We found a negligible qualitative dependence of our results on $W_d$.

Frequencies and normalized eigenvectors of the phonon modes for the calculation of the dynamical structure factor were obtained from Fourier interpolation along the $\Gamma KM$ and $\Gamma M$ paths that we used in our IXS experiments. The integration over the first Brillouin zone in Eq. 2 was performed over a regular grid of 30x30x6 $q$ points. The linewidth $\gamma_{\mathbf{q}j}$ could be derived ab initio from calculations of the contributions of electron-phonon and phonon-phonon coupling to the imaginary part of the phonon self-energy, for example using the EPW and D3 codes in the Quantum Espresso package. However, for reasons of simplicity, we opted for using a value of $0.05\,\mathrm{cm}^{-1}$ in our calculations instead.

The simulated dynamical structure factors for the longitudinal and transverse optical modes corresponding to our experimental setups are shown in Fig. S 2.

In general, the simulated spectra are in good qualitative agreement with our experimental observations and explain the observed signals and relative intensities for the 12 included optical modes. In particular, our simulations correctly predict the branches associated to the longitudinal $E_{2u}$ and $E_{2g}$ modes at the $\Gamma$ point around 35 meV to be inactive for most of the $\Gamma-K$ and $\Gamma-M$ directions in our experimental geometries.[16] This can be understood from the atomic displacement patterns in Tabs. SI–SIII. For these two branches, the two sulfur sublayers in each $MoS_2$ vibrate in opposite phase, causing destructive interference in Eq. 1. For wavevectors with a vanishing out-of-plane component, *i.e.* $\mathbf{q}$=($q_{g1}\,q_{g2}\,0$), the atomic displacements of the sulfur atoms remain perfectly in-plane for most of the $\Gamma-K$ and $\Gamma-M$ high-symmetry lines and the contributions from the vibrating sulfur layers exactly cancel each other out. At the same time, the contributions to Eq. 1 from the equilibrium atomic positions $\mathbf{x}_d$ are equal for all sulfur atoms in a $MoS_2$ layer for the out-of-plane component $q_z$=0. The dynamical structure factor hence vanishes, explaining our observations. As the contributions to the structure factor within each $MoS_2$ layer cancel, this result does not depend on the relative movement (in-phase or counter-phase) of the two $MoS_2$ layers that is the difference between the $E_{2u}$ and $E_{1g}$ modes at $\Gamma$. From our simulations, it also does not depend on the Bragg peak used in the measurements as long as the $z$-component of the phonon wavevector is zero.

On the other hand, our DFT calculations suggest that the dispersion of the optical modes is very weak in out-of-plane, *i.e.* , $\Gamma-A$ direction. This feature could be exploited in order to gain experimental access to the full dispersion of the longitudinal $E^{\Gamma}_{2u}/E^{\Gamma}_{1g}$ branches: a significant out-of-plane component of the wavevector should break the symmetry of the vibration of the two sulfur sublayers in each of the $MoS_2$ layers and lift the destructive interference. Alternatively, one could attempt to break the symmetry of the contributions $e^{i(\mathbf{G}_{hkl}+\mathbf{q})\cdot\mathbf{x}_d}$ in Eq. 1 from the equilibrium positions of the sulfur atoms by sattering the X-rays off lattice planes ($h\,k\,l$) with $l\neq$0. Figure S 3 shows the simulated dynamical structure factors for a selection of Bragg peaks in $\Gamma-M$ and "$\Gamma'-M'$" (with an offset $q_z$=$\frac{1}{4}$) direction. In all cases, breaking of the sulfur sublayer symmetry activates the longitudinal $E^{\Gamma}_{1g}$ or the longitudinal $E^{\Gamma}_{2u}$. The similarity of the results for $q_z$=0 and $q_z=\frac{1}{4}$ suggest that the activation mainly arises from a symmetry breaking of the phase factors from the equilibrium atomic positions, while the contribution from symmetry breaking of the displacement patterns is comparatively small. Depending on the choice of Bragg peak used for IXS, the phase factors $e^{i(\mathbf{G}_{hkl}+\mathbf{q})\cdot\mathbf{x}_d}$ can cause destructive interference between the sulfur sublayers, hence lowering or even extinguishing the scattering intensity, or can cause constructive interference. A choice of Bragg peak that properly aligns the signs of the phase factors from the equilibrium atomic positions with the signs of the corresponding contributions from the atomic displacement, $(\mathbf{G}_{hkl}+\mathbf{q})\cdot\mathbf{e}_{\mathbf{q}jd}$, hence should make the longitudinal $E_{2u}$ and $E_{1g}$ branches experimentally accessible along the $\Gamma-K$ and $\Gamma-M$ paths in future experiments.

This approach is not necessary for the *transverse* $E^{\Gamma}_{2u}$ and $E^{\Gamma}_{1g}$ branches. For these modes, the displacements of the sulfur atoms gain a significant out-of-plane component for wavevectors away from the $\Gamma$ point, which causes a natural symmetry breaking of the contributions from the atomic displacement patterns. The two modes hence behave similarly to the ZO modes and contribute to IXS for a Bragg peak with an out-of-plane component, in case of our experiments ($k\,k\,l$)=(0 0 12). As our simulations suggest, ($k\,k\,l$)=(2 2 2) or similar combinations of $q_{g1}$ and $q_{g2}$ suitable for transverse modes, might work as well or even better along the $\Gamma-K$ and $\Gamma-M$ direction. The situation reverses in the vicinity of the $K$ point: here, the transverse $E_{2u}$ and $E_{1g}$ modes revert back to completely in-plane displacement patterns, while the longitudinal modes evolve into pure out-of-plane vibrations, see Tab. S II. This causes an apparent crossing of the

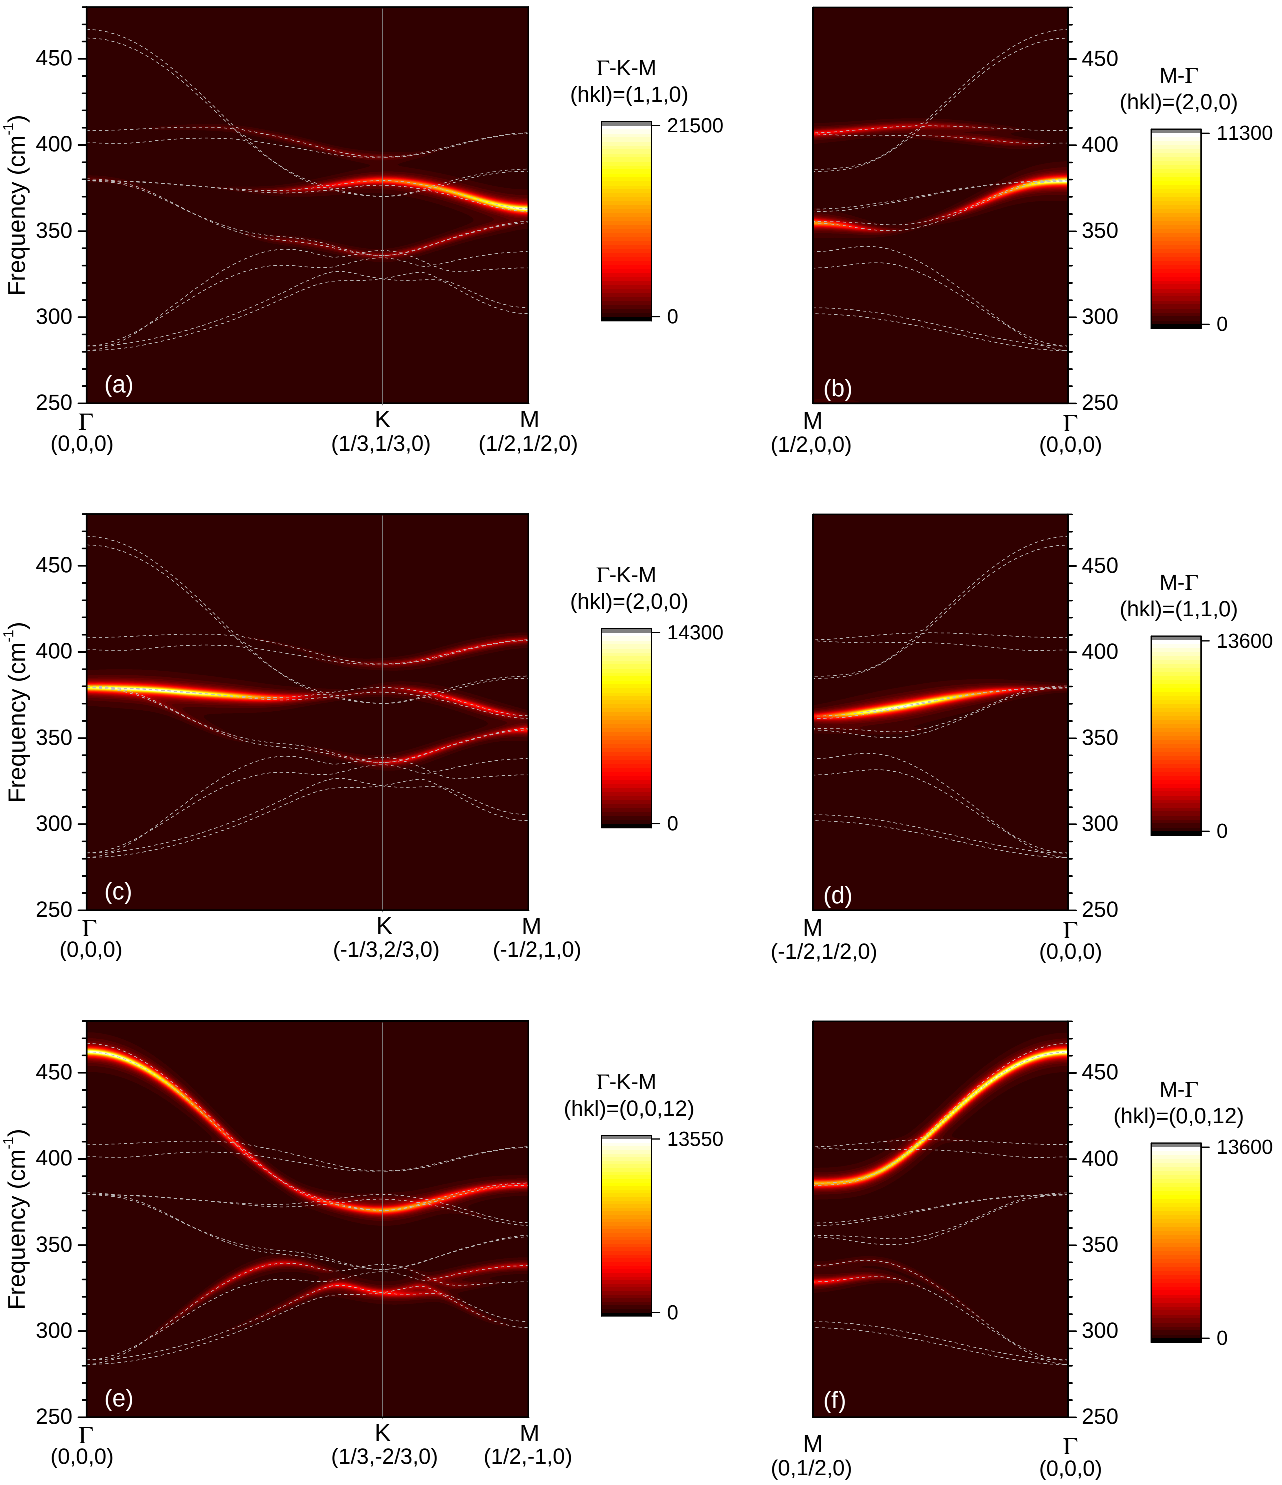


FIG. S 2: Simulated dynamical structure factors for the Bragg peaks and paths in reciprocal space used in our IXS experiments. The phonon dispersion of the optical branches from our DFT calculations is shown as an overlay (dashed lines). The intensity is given in arbitrary units and is meaningful for comparison of the relative scattering intensity between the different experimental geometries.

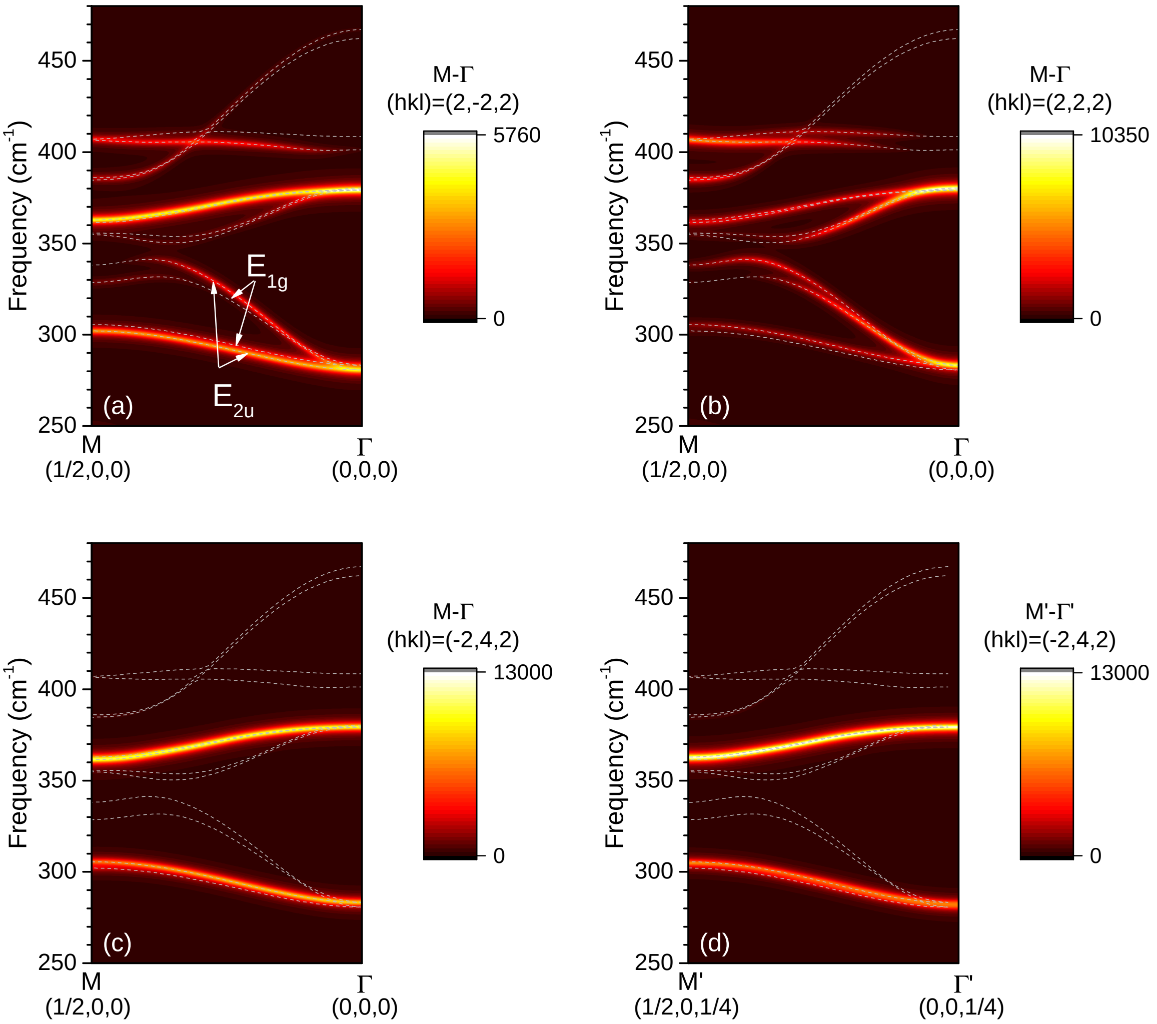


FIG. S 3: Dynamical structure factors for a selection of experimental geometries that might yield scattering contributions from the Davydov pair of branches associated to the longitudinal $E_{2u}$ and $E_{1g}$ modes at the $\Gamma$ point, which we did not observe in our experiments (except near the $K$ point). The scattering intensity shows a strong qualitative and quantitative dependence of the chosen Bragg peak, while the effect of symmetry breaking through an out-of-plane offset of the phonon wavevectors is small.

transverse and longitudinal $E_{2u}^{\Gamma}$ and $E_{1g}^{\Gamma}$ branches close to the $K$ point in both IXS experiments and the simulated dynamical structure factor in Fig. S 2 (e). However, the calculated dispersion and the evolution of the atomic displacement patterns along the $\Gamma - K$ path suggest that this apparent crossing is an actual anti-crossing and that the scattering intensity is transfered from the (pseudo-)transverse modes to the (pseudo-)longitudinal modes in the vicinity of the $K$ point.

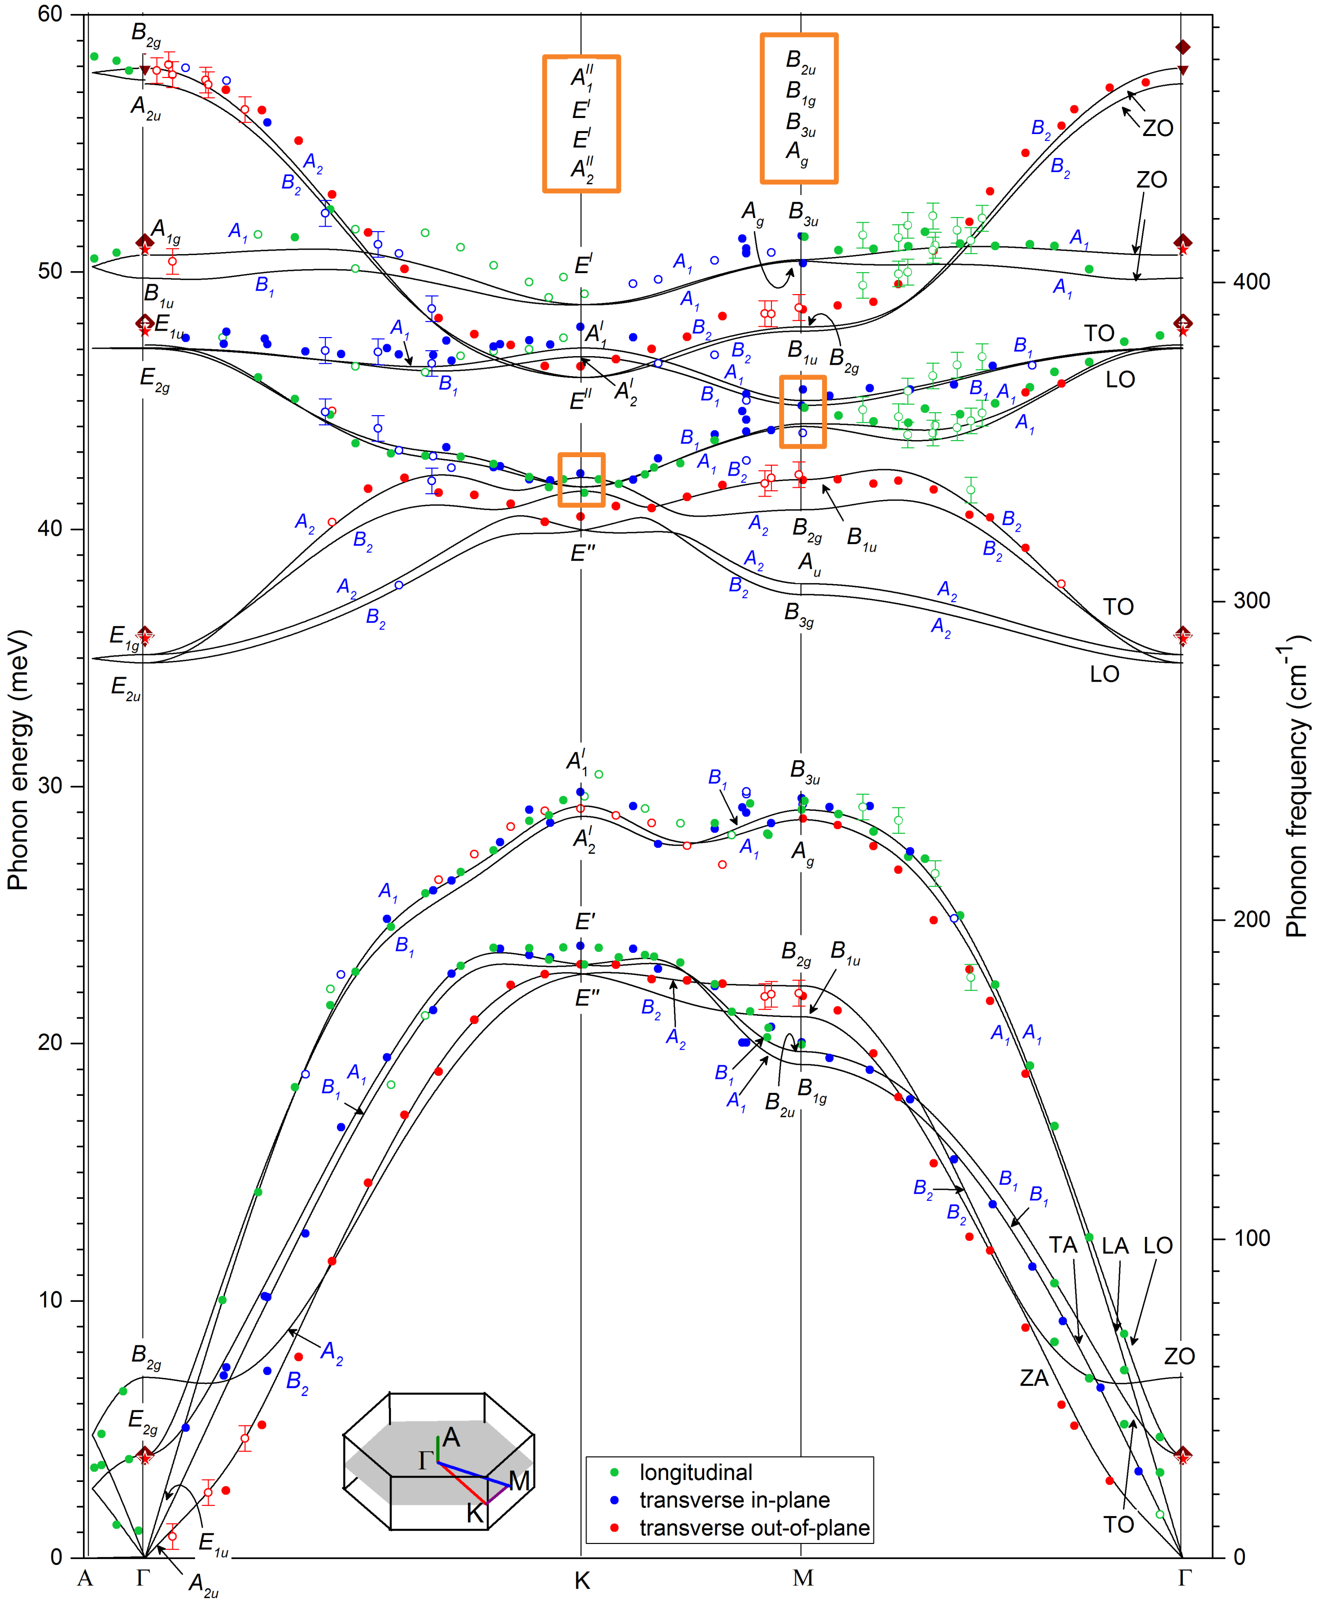


FIG. S4: Dispersion of $MoS_2$ (as of Fig. 2, main text) including the irreducible representations of all branches at the $\Gamma$ ($D_{6h}$), $K$ ($D_{3h}$) and $M$ ($D_{2h}$) points (black) and along the high-symmetry lines ($C_{2v}$, blue). The irreducible representations at the high-symmetry points can be directly derived from the displacement patterns, see Tables S I-III; for correlations between the group $D_{6h}$ and its subgroups $D_{3h}$, $D_{2h}$, and $C_{2v}$, see any text book on group theory or Ref. [13] for the directly related example of the hexagonal Brillouin zone of graphene.

TABLE S I: Phonon eigenvectors of $MoS_2$ at the Γ point. Frames surround Davydov pairs. For each phonon the projections onto the planes depicted in the panel on the bottom right are shown.

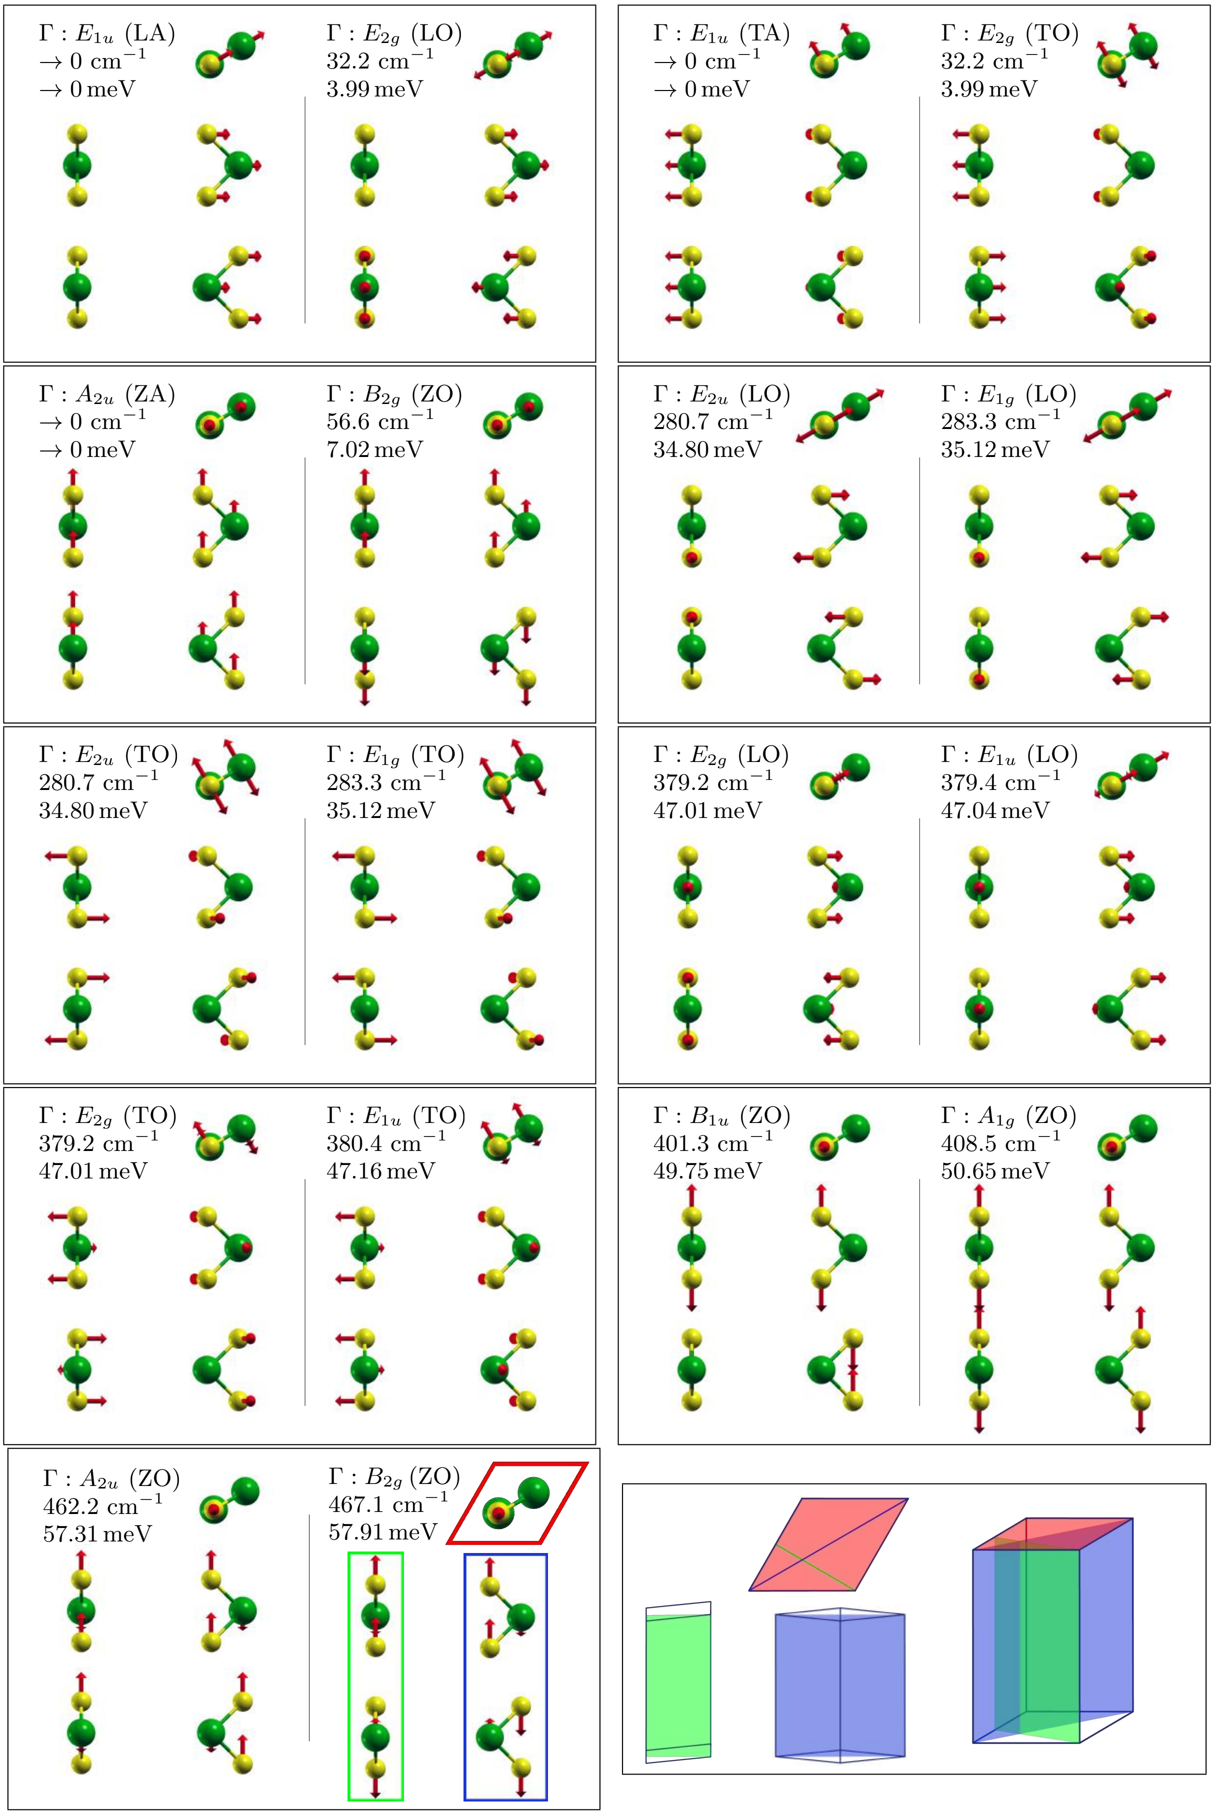

TABLE S II: Eigenvectors of the $MoS_2$ phonons at the $K$ point. Layout according to Tab. S I.

| | | |
|---|---|---|
| $K : E''$<br>$\Gamma : B_{2g}$ (ZO)<br>183.1 cm$^{-1}$<br>22.70 meV<br>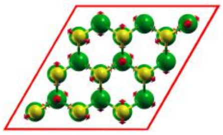<br>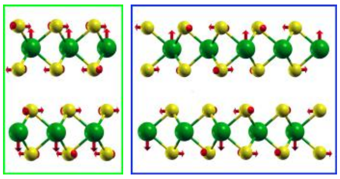 | $K : E''$<br>$\Gamma : A_{2u}$ (ZA)<br>183.1 cm$^{-1}$<br>22.70 meV<br>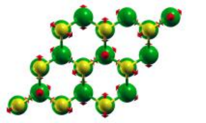<br>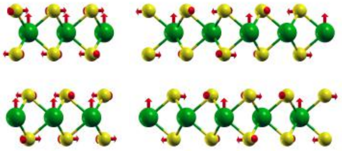 | $K : E'$<br>$\Gamma : E_{1u}$ (TA)<br>186.0 cm$^{-1}$<br>23.06 meV<br>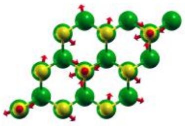<br>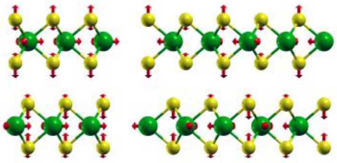 |
| $K : A_2'$<br>$\Gamma : E_{2g}$ (LO)<br>232.5 cm$^{-1}$<br>28.82 meV<br>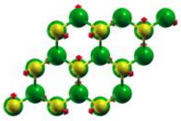<br>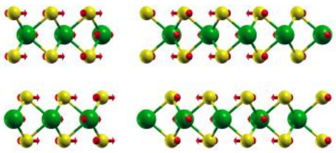 | $K : A_1'$<br>$\Gamma : A_{1u}$ (LA)<br>235.8 cm$^{-1}$<br>29.24 meV<br>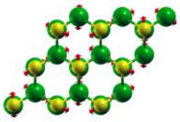<br>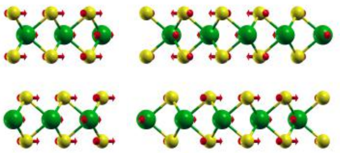 | $K : E'$<br>$\Gamma : E_{2g}$ (TO)<br>186.0 cm$^{-1}$<br>23.06 meV<br>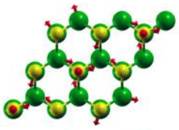<br>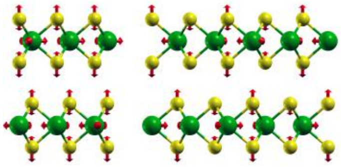 |
| $K : E''$<br>$\Gamma : E_{2u}$ (LO)<br>322.3 cm$^{-1}$<br>39.96 meV<br>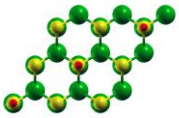<br>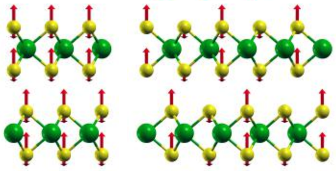 | $K : E''$<br>$\Gamma : E_{1g}$ (LO)<br>322.3 cm$^{-1}$<br>39.96 meV<br>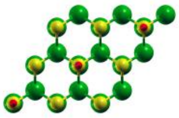<br>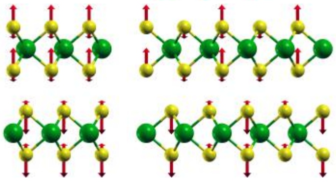 | $K : E'$<br>$\Gamma : E_{1u}$ (LO)<br>335.9 cm$^{-1}$<br>41.65 meV<br>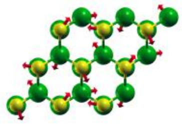<br>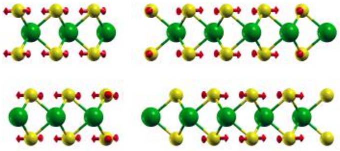 |
| $K : A_1''$<br>$\Gamma : E_{2u}$ (TO)<br>339.0 cm$^{-1}$<br>42.03 meV<br>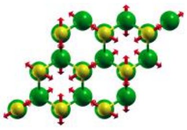<br>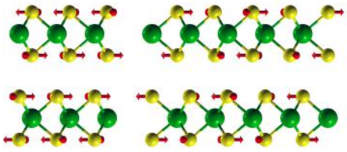 | $K : A_2''$<br>$\Gamma : E_{1g}$ (TO)<br>334.5 cm$^{-1}$<br>41.47 meV<br>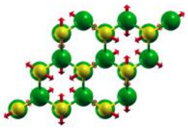<br>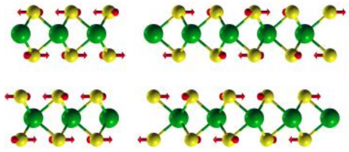 | $K : E'$<br>$\Gamma : E_{2g}$ (LO)<br>335.9 cm$^{-1}$<br>41.65 meV<br>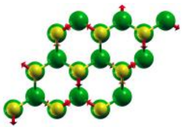<br>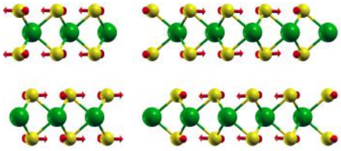 |
| $K : E''$<br>$\Gamma : B_{2g}$ (ZO)<br>370.1 cm$^{-1}$<br>45.89 meV<br>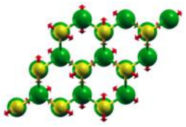<br>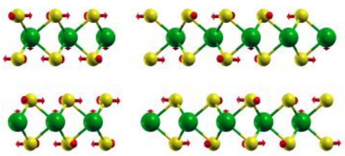 | $K : E''$<br>$\Gamma : A_{2u}$ (ZO)<br>370.1 cm$^{-1}$<br>45.89 meV<br>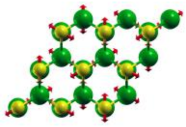<br>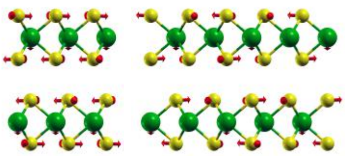 | $K : E'$<br>$\Gamma : B_{1u}$ (ZO)<br>393.0 cm$^{-1}$<br>48.73 meV<br>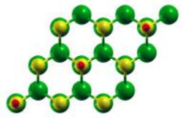<br>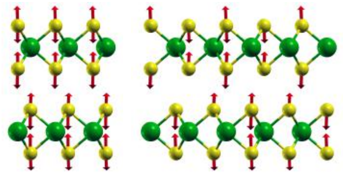 |
| $K : A_2'$<br>$\Gamma : E_{1u}$ (TO)<br>376.7 cm$^{-1}$<br>46.70 meV<br>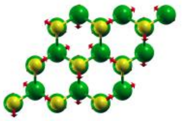<br>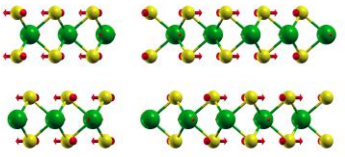 | $K : A_1'$<br>$\Gamma : E_{2g}$ (TO)<br>379.4 cm$^{-1}$<br>47.04 meV<br>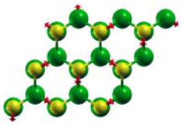<br>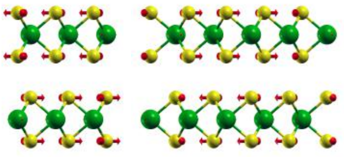 | $K : E'$<br>$\Gamma : A_{1g}$ (ZO)<br>393.0 cm$^{-1}$<br>48.73 meV<br>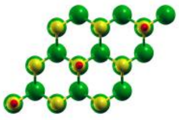<br>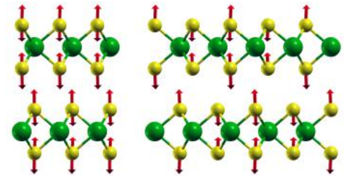 |

TABLE S III: Eigenvectors of the $MoS_2$ phonons at the $M$ point. Layout according to Tab. S I.

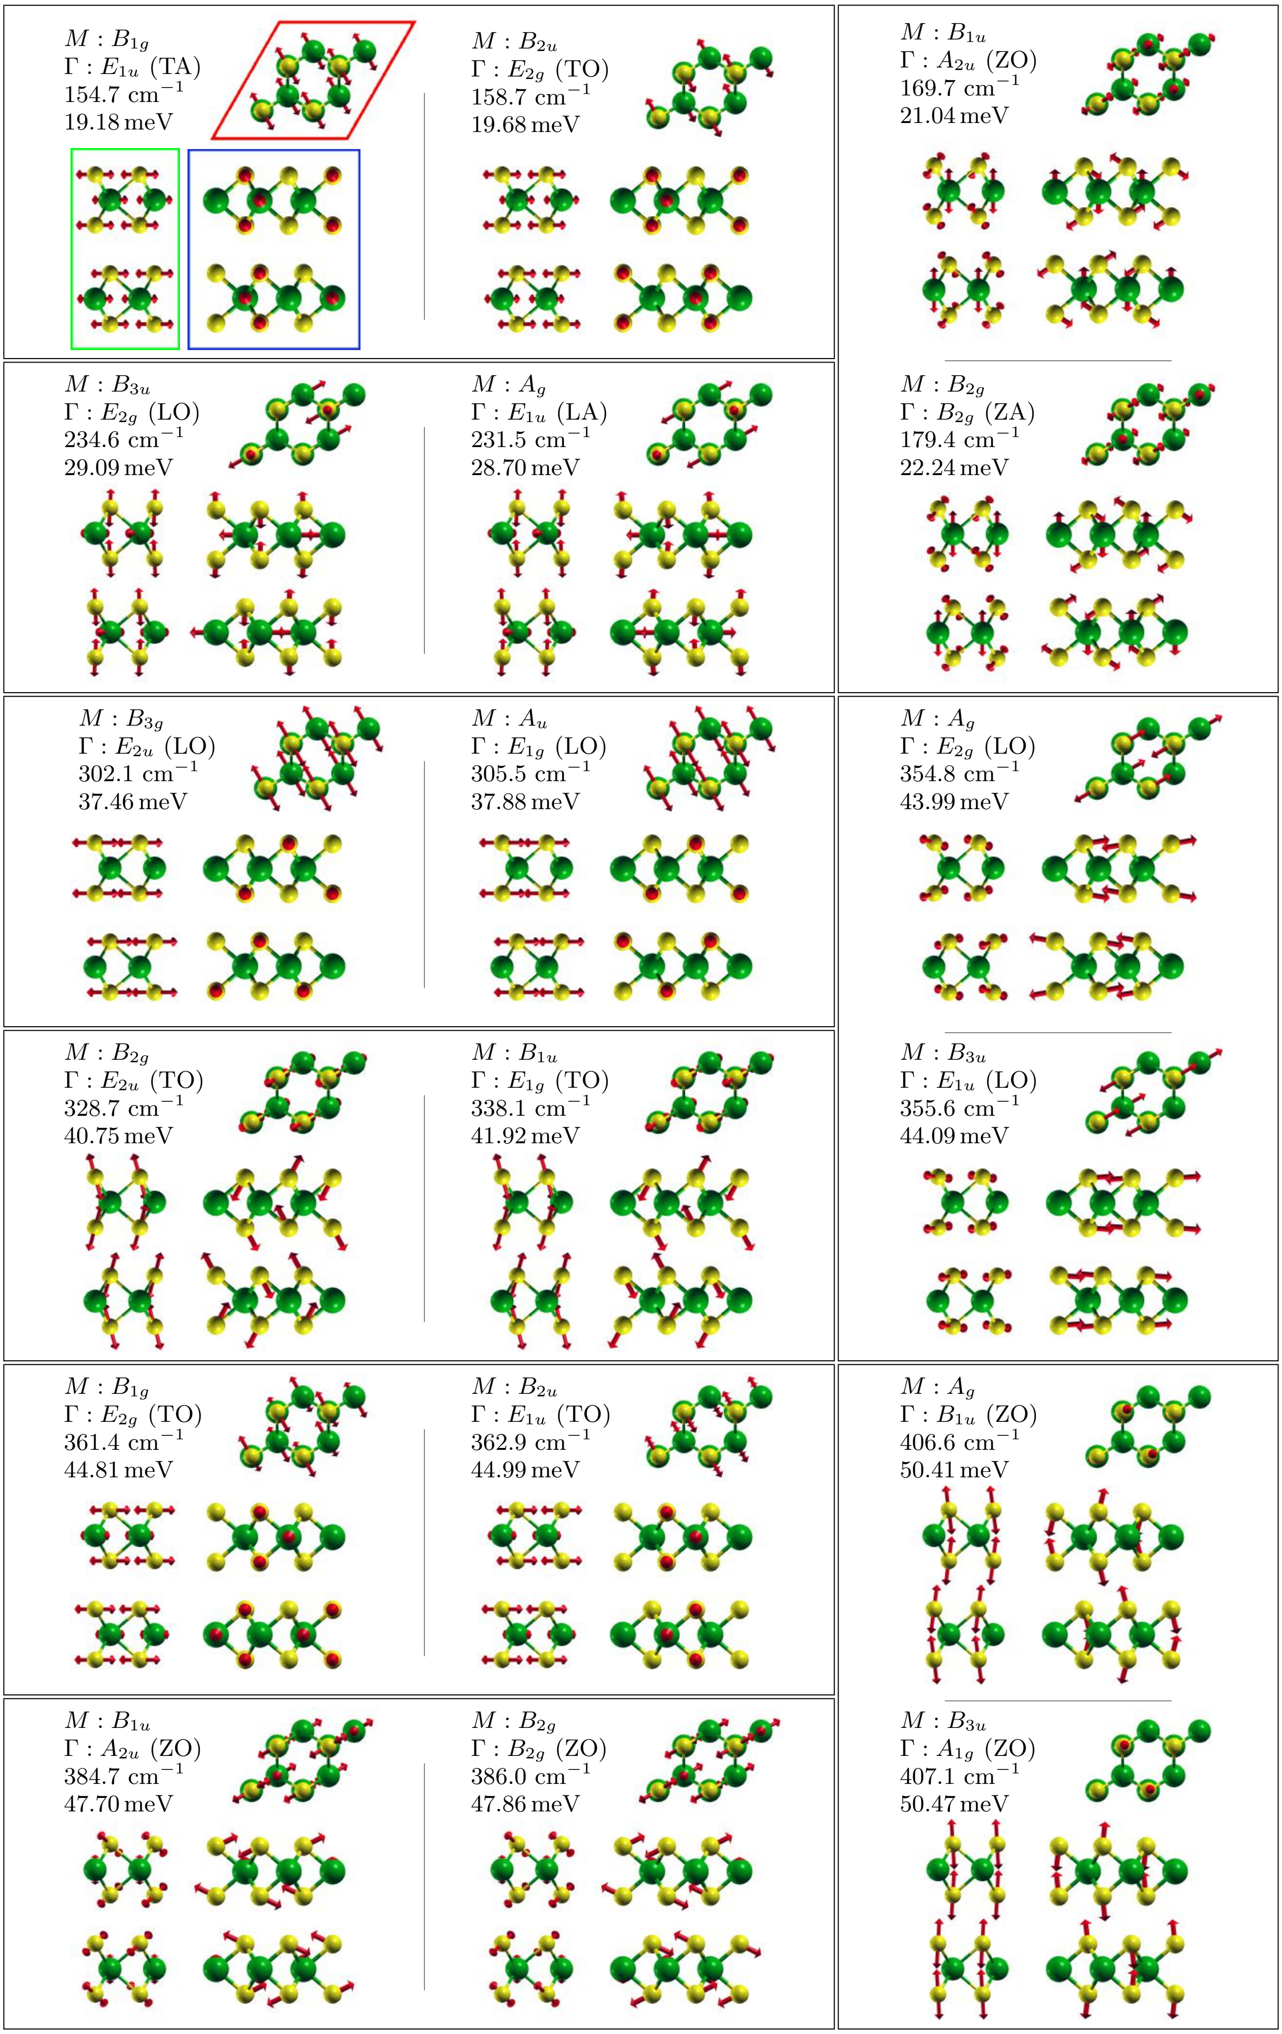

### Comparison of the phonon dispersion obtained by IXS with data from the literature

Despite the importance of the phonon dispersion for the evaluation of mechanical and elastic properties, thermal transport as well as charge-carrier dynamics, phonon-assisted optical excitations and many more, only few experimental values are known for any TMDC. For $MoS_2$, only two measurements of parts of the dispersion have been reported in the literature, to the best of our knowledge.

We compare the dispersion obtained by IXS with the previously reported measurements by electron energy loss spectroscopy (EELS, Fig. S 6, open circles) [14]. The acoustic branches from the EELS measurements deviate significantly from the data obtained by IXS as well as the calculations. As EELS is a surface sensitive technique, one might think that the difference is due to surface defects or reconstruction. However, in a layered material such a large difference between layers near the surface and layers within the bulk seems rather unlikely. We note that the slope of the acoustic branches is by approximately a factor of two different between the EELS and IXS data.

The inelastic neutron scattering (INS) data (Fig. S 6, open squares) [15], on the other hand, are in excellent agreement with the IXS data for the acoustic branches.

A good agreement can be found for the optical branches in the vicinity of the Γ point, however, energies and assignment of some branches deviate close to the $M$ point. An anti-crossing [label (a)] and a crossing of branches [label (b)] can be ruled out by analysis of the selection rules in IXS measurements.

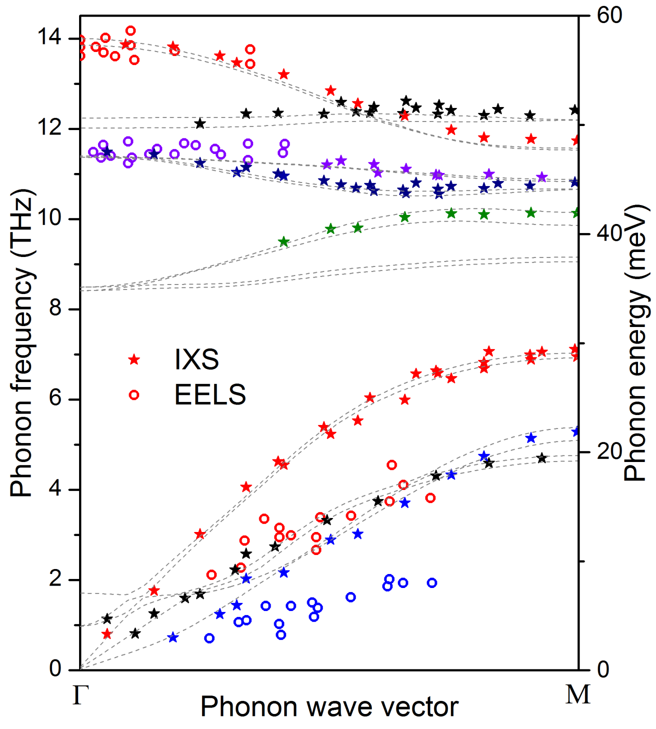


FIG. S 5: Comparison of our IXS data (stars) with EELS measurements of Ref. [14](open circles). Colors depict different branches. Dashed grey lines depict our calculations as a guidance to distinguish different branches.

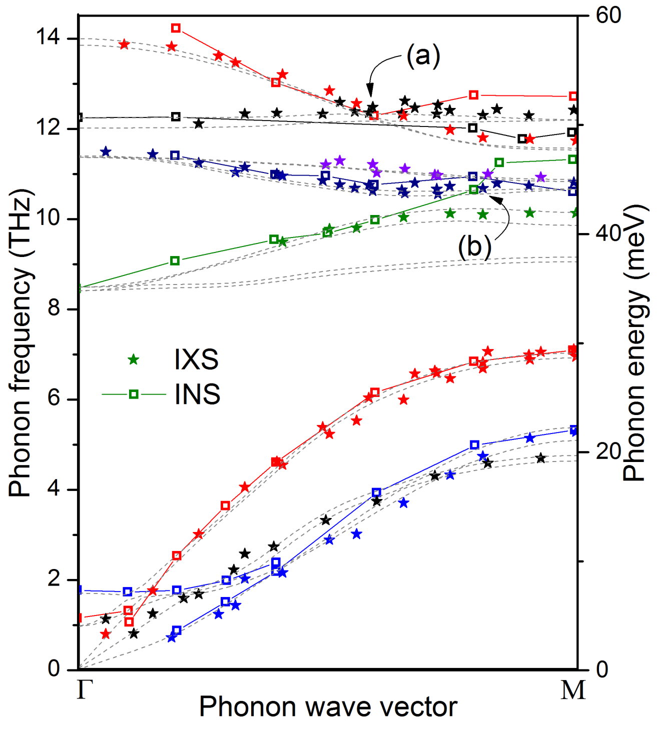


FIG. S 6: Comparison of our IXS data (stars) with INS measurements of Ref. [15] (open squares, connected by lines). Colors depict different branches. Dashed grey lines depict our calculations as a guidance to distinguish different branches.

* Electronic address: ht07@physik.tu-berlin.de

[1] Baron, A. *et al.* An X-ray scattering beamline for studying dynamics. *J. of Phys. Chem. Sol.* **61**, 461–465 (2000).
[2] Giannozzi, P. *et al.* Quantum espresso: a modular and open-source software project for quantum simulations of materials. *J. Phys.: Cond. Mat.* **21**, 395502 (2009).
[3] Grimme, S., Ehrlich, S. & Goerigk, K. Effect of the damping function in dispersion corrected density functional theory. *J. Comput. Chem.* **32**, 1456 (2011).
[4] Gillen, R. & Maultzsch, J. Light-matter interactions in two-dimensional transition metal dichalcogenides: Dominant excitonic transitions in mono- and few-layer $MoX_2$ and band nesting. *IEEE J. Sel. Top. Quantum Electron.* **23**, 219–230 (2017).
[5] Gillen, R. & Maultzsch, J. Interlayer excitons in $MoSe_2/WSe_2$ heterostructures from first principles. *Phys. Rev. B* **97**, 165306 (2018).
[6] Tyborski, C. *et al.* Electronic and vibrational properties of diamondoid oligomers. *J. Phys. Chem. C* **121**, 27082–27088 (2017).
[7] Hamann, D. R. Optimized norm-conserving Vanderbilt pseudopotentials. *Phys. Rev. B* **88**, 085117 (2013).
[8] van Setten, M. J. *et al.* The PseudoDojo: Training and grading a 85 element optimized norm-conserving pseudopotential table. *Com. Phys. Comm.* **226**, 39–54 (2018).
[9] Mignuzzi, S. *et al.* Effect of disorder on Raman scattering of single-layer $MoS_2$. *Phys. Rev. B* **91**, 1–7 (2015).
[10] Guo, H. *et al.* Resonant raman spectroscopy study of swift heavy ion irradiated $MoS_2$. *Nucl. Instrum. Methods Phys. Res.* **381**, 1 – 5 (2016).
[11] Baron, A. Q. R. Phonons in crystals using inelastic X-ray scattering. *J. Spectr. Soc. Jap.* **58**, 205 (2009).
[12] Fåk, B. & Dorner, B. Phonon line shapes and excitation energies. *Physica* **234-236**, 1107 – 1108 (1997).
[13] Reich, S., Thomsen, C. & Maultzsch, J. *Carbon nanotubes: basic concepts and physical properties* (Weinheim-VCH, 2004).
[14] Bertrand, P. A. Surface-phonon dispersion of $MoS_2$. *Phys. Rev. B* **44**, 5745–5749 (1991).
[15] Wakabayashi, N., Smith, H. G. & Nicklow, R. M. Lattice dynamics of hexagonal $MoS_2$ studied by neutron scattering. *Phys. Rev. B* **12**, 659–663 (1975).
[16] For simplicity, we use the irreducible representations at the Γ point for labeling the entire branch inside the Brillouin zone. Where this is ambiguous, we add a superscript "Γ" to emphasize that this labeling is strictly correct only at the Γ point. For a correct symmetry assignment at the $K$ and $M$ points, see Tab. 1 in the main text and Tabs. S I-S III.
